# Supplementary material for: Exploring the Potential of Large Foundation Models for Open-Vocabulary HOI Detection
Source: arXiv:2404.06194 source file (2024-04-10)
Supplement: Supplementary file 1 [file X_suppl.tex]

% \clearpage
\setcounter{page}{1}
% \maketitlesupplementary

In this supplementary material, we offer a more comprehensive assessment of our proposed CMD-SE. In Section~\ref{sec:supp-ablation}, we further investigate the multi-level decoding mechanism and the effect of different descriptions on our model. In Section~\ref{sec:hico-to-swig}, we further analyze the generalizability of our \modelname by comparing it with the previous state-of-the-art zero-shot HOI detector. In Section~\ref{sec:supp-detail}, we provide additional details regarding the implementation of the proposed approach. In Section~\ref{sec:supp-qualitative} we present more qualitative results on images in the wild. In Section~\ref{sec:supp-limitation} we discuss the limitations and potential future directions of our work.

\section{Ablation Study}
\label{sec:supp-ablation}

In this section, we empirically investigate the sensitivity of the proposed method to the multi-level decoding mechanism and the effect of different description on the open-vocabulary SWIG-HOI dataset. Specifically, besides the four aspects of \modelname we have discussed in section 4.3, we further ablate on (1) utilizing different levels of feature maps to decode HOIs and (2) the importance of different descriptions. 

\noindent \textbf{The multi-level decoding mechanism.}
As shown in Table~\ref{tab:ablation-level}, utilizing the feature maps from level $\{6, 9, 12\}$ brings a 0.73\% mAP gain on all categories compared with utilizing the feature maps from level $\{9, 12\}$. It is worth noting that the performance on HOIs with large distances improves by a large margin~(4.69\%), showing the effectiveness of utilizing multi-level feature maps to model HOIs with different distances. 
Furthermore, we empirically find that utilizing more levels of feature maps leads to marginally inferior performance. This shows that utilizing more levels of feature maps might lead to a more challenging optimization during the training process. Therefore, in the main paper, we use the feature maps from level $\{6, 9, 12\}$ by default to report all experimental results unless otherwise specified.

\noindent \textbf{The importance of different descriptions.}
(1) \textit{HOI description:} besides using the annotated verb/object definitions in main paper~(line 1 of Table 6) as HOI description, we try 2 different prompts for querying the LLM: ``Knowledge retrieve for HOI'', and ``Describe the visual appearance of HOI''~(lines 2\&3 of Table~\ref{tab:ablation-prompts}). We observe that ``Knowledge Retrieval'' often includes redundant information lacking relevance to visual cues (e.g., "a common recreational activity"), ``Visual Appearance'' also performs worse compared to ours, suggesting that the underlying states of body parts offer a more broadly applicable comprehension of HOI concepts. 
(2) \textit{Bodypart description:} To better understand the importance of body parts description, we experiment with a subset of body parts~(last row), yielding inferior results compared to using all body parts. This indicates the visual cues from multiple body parts provide complementary and valuable information for open-vocabulary HOID.

\section{Comparative Analysis of Open Vocabulary and Zero-shot HOI Detectors}
\label{sec:hico-to-swig}

% \yang{I will suggest directly link this section with the experiment in Table 2 main text. add a paragraph, starts from Table 2 observation ,highlighting in table 2 all open vocabulary method numbers fall behind zero-shot methods, i.e., it is not a fair comparison. to enable a controlled comparison in dealing with unseen objects in a fair manner, we conduct the following experiment, etc. MAYBE also think whether you want to change a subsection name }

We observe from Table 2 of the main text that all open vocabulary methods perform worse than zero-shot methods on the HICO-DET dataset. However, this comparison is not entirely fair because the zero-shot methods depend on a DETR architecture and often use pretrained weights from COCO~\cite{lin2014COCO}\footnote{The COCO pretraining implicitly encompasses all object categories present in HICO-DET.}. To enable a controlled comparison in dealing with unseen objects in a fair manner, we conduct the following experiment to analyze the generalizability of our model and the previous state-of-the-art zero-shot HOI detector~\cite{ning2023hoiclip}. Specifically, we train both methods on the default setting of the HICO-DET dataset and evaluate their performance on a subset of the SWIG-HOI test set. We randomly select a few classes from the SWIG-HOI test set for evaluation.
As shown in Table~\ref{tab:hico-to-swig}, our proposed method outperforms HOICLIP~\cite{ning2023hoiclip} by 5.62\% and 4.79\% mAP when selecting 20 or 50 classes, respectively. It is worth noting that interactions in SWIG-HOI may involve arbitrary object categories that are not present in the COCO dataset, which is closer to an open-world scenario. Previous methods that rely on a pretrained DETR~\cite{carion2020DETR} exhibit inferior performance when directly applied to SWIG-HOI. In contrast, our proposed CMD-SE, which does not rely on a pretrained detector, demonstrates the greater potential for detecting HOIs in open-world scenarios.

\section{Implementation Details}
\label{sec:supp-detail}

In this section, we present a comprehensive description of the implementation details of our model.
Our model is built upon the pretrained CLIP and all its parameters are frozen during training. Following the previous work~\cite{wang2022_THID}, we employ the ViT-B/16 version as our visual encoder to ensure a fair comparison, which processes a 224 $\times$ 224 $\times$ 3 image as input. During training, we first apply a few data augmentation techniques, including RandomHorizontalFlip, RandomCrop, and ColorJitter. Then, the augmented images are resized to the CLIP input resolution, \ie, 224 $\times$ 224. The visual encoder consists of a total of 12 layers, and we extract feature maps from levels $\{6, 9, 12\}$, forwarding them to the HOI decoder. The number of layers of the HOI decoder is set to 4. We employ 10 and 25 HOI queries on the SWIG-HOI and HICO-DET datasets, respectively. We set the cost weights $\lambda_b$, $\lambda_{iou}$, $\lambda_{cls}$ and $\lambda_{d}$ to 5, 2, 5, and 5 during training. We use focal loss~\cite{lin2017focal_loss} for interaction classification to counter the imbalance between positive and negative examples. We set $\gamma$ to 2 during inference. We introduce 8 prefix tokens and 2 conjunctive tokens to connect the words of human actions and objects following~\cite{wang2022_THID}. We set the learning rate as $10^{-4}$ and use the Adam optimizer with decoupled weight decay regularization. We train our model for 80 epochs with a batch size of 128 on 2 A100 GPUs. 

\section{Qualitative Examples in The Wild}
\label{sec:supp-qualitative}

\begin{figure*}
  \centering  
    \begin{subfigure}{0.24\linewidth}
    \includegraphics[width=0.99\linewidth ]{figures/supp/kicking_person.jpg}
    \caption{kicking person.}
    \label{fig:supp-a}
  \end{subfigure}
   \hfill
  \begin{subfigure}{0.24\linewidth}
    \includegraphics[width=0.99\linewidth ]{figures/supp/drinking_drinking_glass.jpg}
    \caption{drinking drinking-glass.}
    \label{fig:supp-b}
  \end{subfigure}
   \hfill
  \begin{subfigure}{0.24\linewidth}
    \includegraphics[width=0.99\linewidth ]{figures/supp/talking_telephone.jpg}
    \caption{talking telephone.}
    \label{fig:supp-c}
  \end{subfigure}
   \hfill
  \begin{subfigure}{0.24\linewidth}
    \includegraphics[width=0.99\linewidth ]{figures/supp/photographing_camera.jpg}
    \caption{photographing camera.}
    \label{fig:supp-d}
  \end{subfigure}
  \\
  \begin{subfigure}{0.24\linewidth}
    \includegraphics[width=0.99\linewidth ]{figures/supp/shooting_shotgun.jpg}
    \caption{shooting shotgun.}
    \label{fig:supp-e}
  \end{subfigure}
   \hfill
  \begin{subfigure}{0.24\linewidth}
    \includegraphics[width=0.99\linewidth ]{figures/supp/riding_horse.jpg}
    \caption{riding horse.}
    \label{fig:supp-f}
  \end{subfigure}
  \hfill
  \begin{subfigure}{0.24\linewidth}
    \includegraphics[width=0.99\linewidth ]{figures/supp/reading_book.jpg}
    \caption{reading book.}
    \label{fig:supp-g}
  \end{subfigure}
   \hfill
  \begin{subfigure}{0.24\linewidth}
    \includegraphics[width=0.99\linewidth ]{figures/supp/smoking_cigarette.jpg}
    \caption{smoking cigarette.}
    \label{fig:supp-h}
  \end{subfigure}

  \caption{Qualitative results of our method on wild data.}
  \label{fig:short}
\end{figure*}

\begin{table}
  \centering
  \begin{tabular}{@{}cccccc@{}}
    \toprule
    $\mathbb{L}$    & Small & Large  & Seen & Unseen & Full \\
    \midrule
    \{9, 12\}       & 15.26 & 13.30 & 16.79 & 10.05 & 15.09 \\
    \{6, 9, 12\}    & \textbf{15.20} & \textbf{17.35} & \textbf{16.79} & \textbf{10.70} & \textbf{15.26} \\
    % \{3, 6, 9, 12\} & 15.44 & 17.28 & 17.07 & 10.35 & 15.38 \\
    \{3, 6, 9, 12\} & 15.13 & 16.93 & 16.73 & 10.14 & 15.07 \\
    \bottomrule
  \end{tabular}
  \caption{Ablation on the multi-level decoding mechanism. $\mathbb{L}$: the levels of feature maps used for decoding. Small: HOIs with small distances~($\leq$0.33). Large: HOIs with large distances~($\geq$0.67).}
  \label{tab:ablation-level}
\end{table}

\begin{table}
  \centering
  \begin{tabular}{@{}lc@{}}
    \toprule
    Prompts & Unseen \\
    \midrule
    None    &  9.32 \\
    Knowledge Retrieval &  9.85\small[\textcolor[RGB]{255,0,0}{+0.53}] \\
    Visual Appearance   & 10.27\small[\textcolor[RGB]{255,0,0}{+0.95}] \\
    Body Part       & \textbf{10.70}\small[\textcolor[RGB]{255,0,0}{+1.38}]  \\ 
    Subset of Body Part & 10.25\small[\textcolor[RGB]{255,0,0}{+0.93}]  \\           
    \bottomrule
  \end{tabular}
  \caption{Importance of different descriptions.}
  \label{tab:ablation-prompts}
\end{table}

\begin{table}
  \centering
  \begin{tabular}{@{}ccc@{}}
    \toprule
    Method    & \#(Classes) & mAP \\
    \midrule
    HOICLIP~\cite{ning2023hoiclip} & 20 & 7.41 \\
    \modelname (Ours)              & 20 & \textbf{13.03}\\
    \hline
    HOICLIP~\cite{ning2023hoiclip} & 50 & 4.39 \\
    \modelname (Ours)              & 50 & \textbf{9.18} \\
    \bottomrule
  \end{tabular}
  \caption{Experiments on applying methods trained on HICO-DET to SWIG-HOI dataset. \#(Classes): the number of classes we select on the SWIG-HOI test set.}
  \label{tab:hico-to-swig}
\end{table}

To provide further evidence of the enhanced performance and generalization capabilities of our model, we present additional qualitative results on data in the wild.

\noindent \textbf{Human Body Parts.}
As depicted in Figure~\ref{fig:supp-a} and \ref{fig:supp-b}, our model effectively captures contextual features from image regions containing human body parts, particularly those involved in interactive actions (\eg, legs in ``kicking person," mouth in ``drinking drinking-glass"). It accurately predicts interaction categories based on these extracted features.

\noindent \textbf{Different Distances.} 
Our model demonstrates strong performance across varying distances and scales of human-object interactions, as demonstrated in Figure~\ref{fig:supp-c} and \ref{fig:supp-d}. Whether dealing with small-scale interactions like ``talking telephone" or large-scale interactions like ``photographing camera," our model consistently achieves favorable results.

\noindent \textbf{Different art styles.} 
To assess the model's generalizability to different art styles, we conduct tests using images of video game characters. Figure~\ref{fig:supp-e} and \ref{fig:supp-f} showcase the model's correct predictions of interactions even when presented with out-of-domain images. This demonstrates its commendable performance for images with diverse art styles.

\noindent \textbf{Multiple HOIs.}
We also evaluate the model's ability to detect multiple HOIs in a single image. As shown in Figure~\ref{fig:supp-g} and \ref{fig:supp-h}, our model correctly identifies two different interactions through separate prediction heads. Although the attention patterns of these heads may appear similar, closer inspection reveals that each head actually pays more attention to the objects related to its predictions.

\section{Limitations}
\label{sec:supp-limitation}

Currently, our method is limited in the following two key aspects. Firstly, while we utilize GPT to generate fine-grained descriptions of human body parts for each HOI, our model's ability to distinguish between different HOIs is still constrained by the embedding space of the CLIP text encoder. Secondly, our current approach does not rely on pretrained detectors, which is a strength but may also be a weakness given recent advances in open-vocabulary object detection.
In the future, we will explore ways to utilize more advanced text encoders and integrate high-quality open-vocabulary object detectors into our model. We believe that these improvements will lead to even better performance and make our method more practical for real-world applications.

% \yang{I do not like this limitation, I thought avoid using other pretrained detector is one of your design principle, isn't it?   I will suggest another future work could be rather than human parts; one may also consier object parts or object pose etc.}
